# Supplementary material for: Valley Polarization in Size-Tunable Monolayer Semiconductor Quantum Dots
Source: arXiv:1510.09135 ancillary file (2015-10-30)
Supplement: Supplementary file 1 [file Wei_Arxiv_Supplementary_Information.pdf]

# Supplementary Material for Valley Polarization in Size-Tunable Monolayer Semiconductor Quantum Dots

Guohua Wei,[1] David A. Czaplewski,[2] Erik J. Lenferink,[3] Teodor K. Stanev,[3] Il Woong Jung,[2] and Nathaniel P. Stern[1,3,*]

[1]*Applied Physics Program, Northwestern University, 2145 Sheridan Road, Evanston, IL 60208, USA*

[2]*Center for Nanoscale Materials, Argonne National Laboratory, 9700 S Cass Avenue, Argonne, IL 60439, USA*

[3]*Department of Physics and Astronomy, Northwestern University, 2145 Sheridan Road, Evanston, IL 60208, USA*

## I. FABRICATION

Monolayer $MoS_2$ flakes are obtained using mechanical exfoliation with the Scotchtape technique from a bulk crystal (SPI Supplies). The flakes are dry transferred onto a $SiO_2$/Si substrate with pre-written alignment marks [1, 2]. Identification of monolayer $MoS_2$ is routinely done using atomic force microscopy (AFM), optical contrast, and photoluminescence spectroscopy as described previously [2]. Devices are annealed in an Ar/$H_2$ environment before patterning with electron beam (e-beam) lithography.

QD patterning is performed using a JEOL 9300 electron beam lithography system operating at 100 kV. Pattern writing is only performed on part of each flake to enable control measurements on the unprocessed continuous monolayer from the same $MoS_2$ flake (Fig. S1). Typical optical images of a device are shown in Fig. S1. To reduce exposure damage to the monolayer by the electron beam, larger size rectangular regions with side length $\sim 80$ nm are first patterned by e-beam lithography using positive resist (GL2000) with cold development, illustrated in Fig. S2. A reactive ion etch (RIE) is performed following the e-beam patterning process. The RIE conditions are 20/10 sccm of $CHF_3$/$O_2$ gas flow with 30 W RF power at a pressure of 50 mTorr. The etching time is $10 - 40$ seconds depending on the desired QD size. Fig. S1c,d shows the AFM images of one sample. After RIE etching for 20 s, the QD size is clearly smaller than the initial pattern, enabling control of the final effective QD size. Etching for 10 s is sufficient to remove the monolayer in the region that has been exposed; longer etching times reduce the QD size from the original pattern while rounding the corners. The resist is not removed at the end of processing to prevent destruction of the monolayer QDs.

* n-stern@northwestern.edu

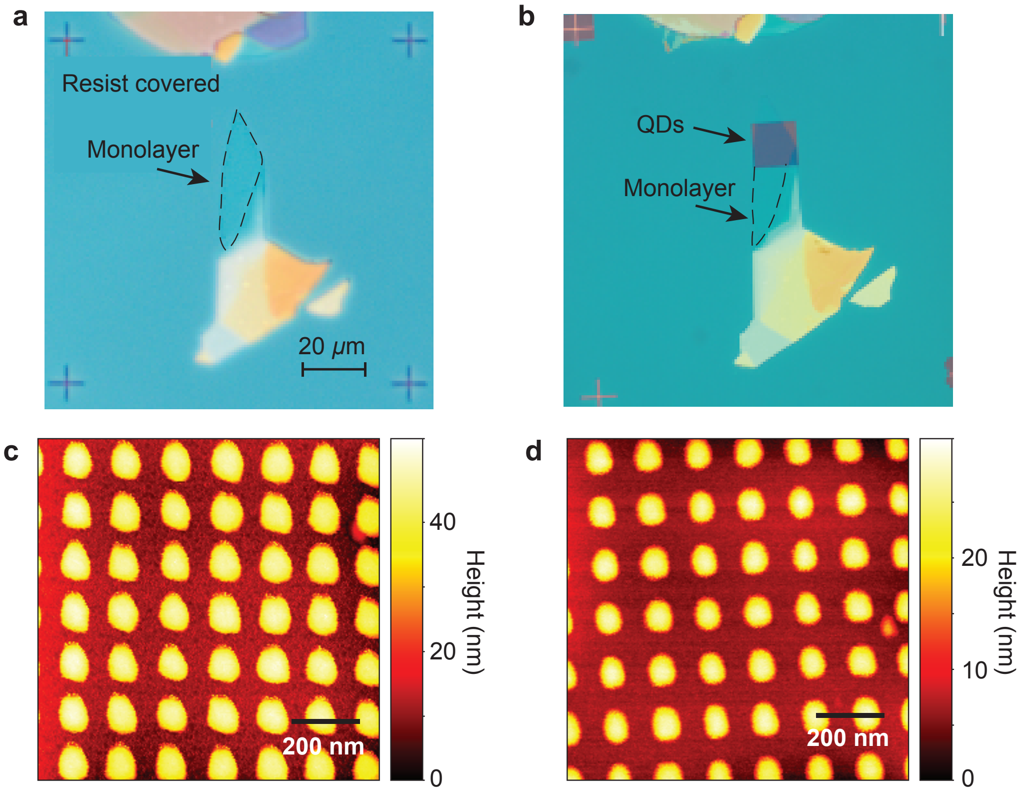


FIG. S1. Optical and AFM images illustrating the fabrication process. **a**, **b** Optical images of the monolayer flake before (**a**) and after (**b**) fabrication. The blue color is the resist layer that covers the top of the sample except in the e-beam patterning region (square). The outline of the monolayer shows that only a part of the monolayer flake has been patterned into QDs. **c**,**d** AFM images of QDs before (**c**) and after (**d**) RIE etching. The 40 nm height reading is because the resist is not removed from the top of the QDs.

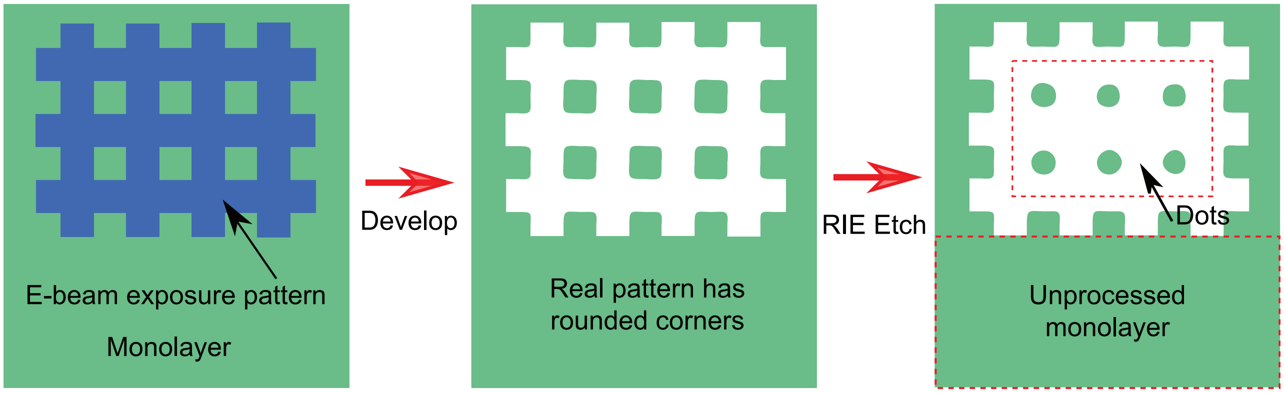


FIG. S2. Illustration of the e-beam lithography process. The arrows show the process steps. A monolayer flake is patterned with lines that criss-cross over a region of the flake. Because of the small size, the square pattern exhibits rounded corners after developing. These large regions with radius of about 40 nm are etched by RIE to make even smaller monolayer dots. The exposed monolayer is removed during this process.

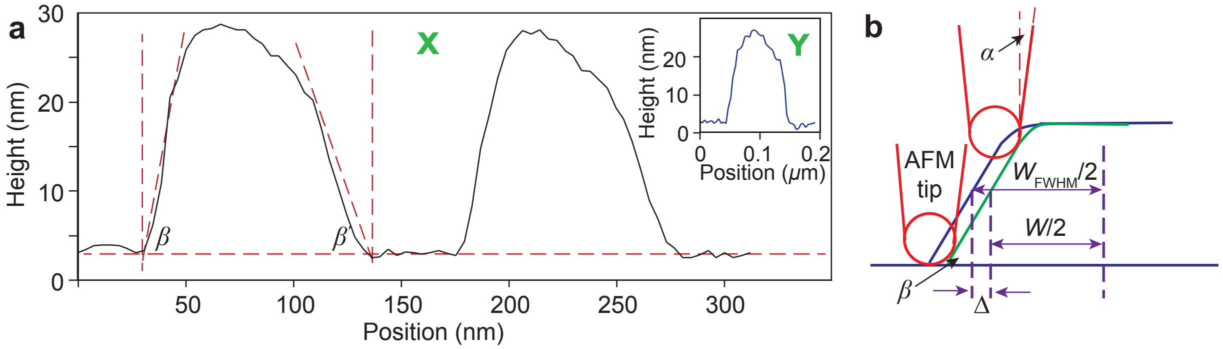


FIG. S3. AFM tip-sample convolution. **a**, The AFM height profile of QDs along the scan direction, labelled $X$. The inset shows a similar profile extracted in the perpendicular direction $Y$. $\beta$ and $\beta'$ are the direction-dependent side wall angles. Slightly asymmetric side wall angles are measured in some AFM scans due to scan speed, but this disappears under symmetric conditions (such as in the extracted $Y$ data). **b**, Schematic of the geometric convolution (blue curve) of the AFM tip radius $R_{\text{tip}}$ with the actual side profile (green curve).

## II. QD SIZE CHARACTERIZATION

QD sizes are measured using AFM. The QD size distribution used in the main text is obtained from image processing using the ImageJ program. In order to characterize the QDs sizes, the area of each QD is measured and converted to an effective radius for the size distribution. The actual size of a monolayer QD differs from that measured directly from image processing of the AFM data. Since the AFM tip has a finite size, the lateral resolution of an AFM scan depends on the tip geometry. The real AFM profile of the QDs is a convolution of the AFM tip profile and the sample geometry that depends on the side wall angle $\beta$ shown in Fig. S3 [3]. Directional asymmetry in the side wall angle is observed due to the AFM scan speed, but this does not impact the conclusions of the typical geometric size correction described here.

In our QDs topped by a photoresist layer, $\beta$ is always smaller than 60°. Since the AFM tip angle is normally smaller than 30°, the tip-sample convolution is determined by the rounding of the AFM tip illustrated in Fig. S3b, in which the measured topography follows the blue curve while the real surface is the green curve. The size of a QD can is characterized by the full width at half height $W_{\text{FWHM}}$. The measured radius $W_{\text{FWHM}}/2$ differs from the actual radius $W/2$ by a geometric correction $\Delta = W_{\text{FWHM}}/ - W/2$. Assuming the AFM tip is rounded with radius of curvature $R_{\text{tip}}$, the measured tip path results in a geometric correction to the true QD radius of $\Delta = R_{\text{tip}} \tan(\beta/2)$. For a typical fresh AFM tip with $R_{\text{tip}} \sim 10$ nm, the correction $\Delta$ is around $3-5$ nm. Since the AFM tip broadens with usage, this correction should be a lower limit on the expected geometric size correction.

As described in the main text and the references, chemical adsorption at the edge in ambient conditions can result in reduction of the effective QD size for determining quantum confinement. Up to $\Delta R \sim 8$ nm is extracted from the exciton energy dependence, which is reasonable due to the combined geometric and chemical mechanisms.

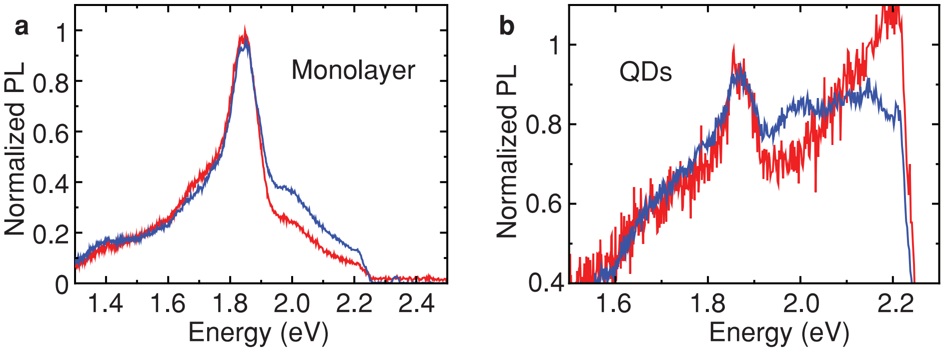


FIG. S4. Device stability over two months. **a**, The red PL spectrum is measured two months after the blue PL spectrum from the same monolayer. **b**, The same measurements for patterned QDs.

## III. DEVICE STABILITY

Unlike nanocrystal QDs and colloidal QD solids, which generally have very short lifetime even in inert environments [4–8], monolayer $MoS_2$ QDs are found to perform consistently over the period of time that we have measured them. Fig. S4 shows PL measurements from the $R = 20$ nm QD sample separated by over two months. The red PL spectra are measured two months after the blue spectra. The PL peak energy and linewidth agree well in both measurements. Similar preservation of performance over many months was also observed from other QD samples. After up to four months of storing a QD device in a desiccator, PL quenching is not observed and the exciton energy shift is reproducible. The relatively long lifetime can be a result of the resist protection of the materials 2D surface.


[1] Castellanos-Gomez, A. *et al.* Deterministic transfer of two-dimensional materials by all-dry viscoelastic stamping. *2D Mater.* **1**, 011002 (2014).

[2] Wei, G., Stanev, T. K., Czaplewski, D. A., Jung, I. W. & Stern, N. P. Silicon-nitride photonic circuits interfaced with monolayer $MoS_2$. *Appl. Phys. Lett.* **107**, 091112 (2015).

[3] Canet-Ferrer, J., Coronado, E., Forment-Aliaga, A. & Pinilla-Cienfuegos, E. Correction of the tip convolution effects in the imaging of nanostructures studied through scanning force microscopy. *Nanotechnology* **25**, 395703 (2014).

[4] Ip, A. H. *et al.* Hybrid passivated colloidal quantum dot solids. *Nature Nanotech.* **7**, 577–582 (2012).

[5] Chuang, C.-H. M., Brown, P. R., Bulović, V. & Bawendi, M. G. Improved performance and stability in quantum dot solar cells through band alignment engineering. *Nature Mater.* **13**, 796–801 (2014).

[6] Ning, Z. *et al.* Air-stable n-type colloidal quantum dot solids. *Nature Mater.* **13**, 822–828 (2014).

[7] Sykora, M. *et al.* Effect of air exposure on surface properties, electronic structure, and carrier relaxation in pbse nanocrystals. *ACS Nano* **4**, 2021–2034 (2010).

[8] Ihly, R., Tolentino, J., Liu, Y., Gibbs, M. & Law, M. The photothermal stability of PbS quantum dot solids. *ACS Nano* **5**, 8175–8186 (2011).
